# Supplementary material for: Parameter tuning and model selection in optimal transport with semi-dual Brenier formulation
Source: arXiv:2112.07275 source file (2023-01-31)
Supplement: Supplementary file 1 [file table_da_supplement.tex]

\begin{tabular}{lcc|cc|cc|cc}
\toprule
{} & \multicolumn{2}{c}{ICNN} & \multicolumn{2}{c}{Sinkhorn} & \multicolumn{2}{c}{SSNB} \\
{} & $\text{acc}(f_{i_1})$ &  $\text{acc}(f_{i_0})$ & $\text{acc}(f_{i_1})$ & $\text{acc}(f_{i_0})$ & $\text{acc}(f_{i_1})$ &  $\text{acc}(f_{i_0})$ \\
\midrule
D/A &          0.5 &   0.47 (2/48) &         0.91 &   0.78 (5/5) &         0.91 &  $\mathbf{0.84}$ (11/11) \\
D/C &         0.54 &   0.43 (2/48) &         0.83 &   0.74 (5/5) &         0.83 &   $\mathbf{0.75}$ (9/11) \\
D/W &         0.52 &  0.28 (11/48) &         0.96 &   0.85 (4/5) &         0.99 &  $\mathbf{0.95}$ (8/11) \\
W/A &         0.48 &  0.25 (17/48) &         0.89 &   $\mathbf{0.78}$ (4/5) &         0.87 &  0.77 (11/11) \\
W/C &          0.4 &   0.2 (13/48) &         0.77 &   0.73 (4/5) &         0.78 &  $\mathbf{0.74}$ (10/11) \\
W/D &         0.62 &   0.51 (2/48) &         0.95 &    0.9 (3/5) &          1.0 &    $\mathbf{1.0}$ (1/11) \\
\bottomrule
\end{tabular}
